# Supplementary material for: Spectral interferometric polarised coherent anti-Stokes Raman spectroscopy
Source: arXiv:1303.5661 source file (2013-03-22)
Supplement: Supplementary file 1 [file SIP-CARS_supp_info.pdf]

# Spectral interferometric polarised coherent anti-Stokes Raman spectroscopy: supplemental information

Brad Littleton,[1] Thomas Kavanagh,[1] Frederic Festy,[2] and David Richards[1]

*[1]Department of Physics, King's College London, Strand, London, WC2R 2LS*
*[2]Biomaterials, Biomimetics and Biophotonics Department,*
*King's College London Dental Institute, Floor 17 Tower Wing,*
*Guy's Hospital, London Bridge, London SE1 9RT, UK*

## I. SIP-CARS SPECTRUM WITH ARBITRARY STOKES AND PUMP/PROBE ELLIPTICITIES

The pump and probe fields are assumed degenerate, and the elliptical polarisations are assumed to have major and minor axes aligned with the $x$- and $y$-axes (as defined is Figure 1(b) main text). The $x$- and $y$-components of the Stokes and pump/probe fields ($E_S$ and $E_p$, respectively) can therefore be written as

$$E_{S_y} = i\varepsilon E_{S_x}, \quad E_{p_y} = i\kappa E_{p_x}$$
$$\text{where} \quad \varepsilon = \tan\theta, \quad \kappa = \tan\phi \tag{1}$$
$$\text{and} \quad E_{S_x} = E_S \cos\theta \quad E_{p_x} = E_p \cos\phi \tag{2}$$

$\theta$ and $\phi$ are as defined in the main paper. The polarisation induced along the $x$- and $y$-axes is then

$$P_x = \left(\chi_{1111} - \kappa^2\chi_{1221} + \kappa\varepsilon\chi_{1122} + \kappa\varepsilon\chi_{1212}\right) E_{p_x}^2 E_{S_x}^* \tag{3}$$
$$P_y = \left(i\kappa\chi_{2121} + i\kappa\chi_{2211} + i\kappa^2\varepsilon\chi_{2222} - i\varepsilon\chi_{2112}\right) E_{p_x}^2 E_{S_x}^* \tag{4}$$

Along the detection axes ($\pm\pi/4$ from the $x$-axis) the induced polarisations are $P_+ = \frac{1}{\sqrt{2}}(P_x + P_y)$ and $P_- = \frac{1}{\sqrt{2}}(P_x - P_y)$, and the difference of the intensities measured along these axes is

$$\Delta S = S_+ - S_- \propto P_x P_y^* + \left(P_x P_y^*\right)^*$$

Substituting (3) and (4), and assuming isotropic symmetry (such that $\chi_{2222} = \chi_{1111}, \chi_{2121} = \chi_{1212}, \chi_{2211} = \chi_{1122}$, and $\chi_{2112} = \chi_{1221}$) this becomes

$$\Delta S \propto 2I_{p_x}^2 I_{S_x}\left(\left(\kappa - \kappa^3\varepsilon^2\right)\mathrm{Im}\left\{\chi_{1111}\left(\chi_{1212}^* + \chi_{1122}^*\right)\right\} + \left(\kappa^4\varepsilon - \varepsilon\right)\mathrm{Im}\left\{\chi_{1111}\chi_{1221}^*\right\} + \left(\kappa\varepsilon^2 - \kappa^3\right)\mathrm{Im}\left\{\chi_{1221}\left(\chi_{1212}^* + \chi_{1122}^*\right)\right\}\right)$$

where $I_i = E_i E_i^*$. Also from isotropic symmetry we have the relation

$$\chi_{1212}^* + \chi_{1122}^* = \chi_{1111}^* - \chi_{1221}^*,$$

which simplies $\Delta S$ to

$$\Delta S \propto 2I_{p_x}^2 I_{S_x}\left[\left(\kappa^3 - \kappa\right)\left(1 + \varepsilon^2\right) + \varepsilon\left(\kappa^4 - 1\right)\right]\mathrm{Im}\left\{\chi_{1111}\chi_{1221}^*\right\}.$$

After substituting for $\varepsilon$ and $\kappa$ from (1), and expressing in terms of the input Stokes and pump/probe field intensities via (2), the expression reduces to

$$\Delta S \propto I_p^2 I_S C(\theta,\phi)\mathrm{Im}\left\{\chi_{1111}\chi_{1221}^*\right\} \tag{5}$$

where

$$C(\theta,\phi) = \frac{1}{2}[\sin(4\phi) + \sin(2\theta) + \sin(2\theta)\cos(4\phi)]$$

The maximum of $\mid C(\theta,\phi) \mid$ is $(1+\sqrt{2})/2$, and occurs at $\theta = \frac{\pi}{4}(4k \pm 1)$, $\phi = \frac{\pi}{16}(8k' \pm 1)$ $(k, k' \in \mathbb{Z})$. For the case of one elliptical and one linear polarisation the maximum amplitudes are

$$\mid C_{max}(\theta, 0) \mid = \frac{1}{2} \quad \text{at}\, \theta = \frac{\pi}{4}(1+2k)$$
$$\mid C_{max}(0, \phi) \mid = \frac{1}{4} \quad \text{at}\, \phi = \frac{\pi}{8}(1+2k)$$

## II. FULL SINGLE-EXPOSURE SIP-CARS SPECTRUM

Figure S1 shows a single-exposure SIP-CARS spectrum for cyclohexane, and its comparison to spontaneous Raman measurements. Strong dispersion in the supercontinuum Stokes field, $I_S$, limited temporal overlap with the pump; consequently most of the energy in the anti-Stokes field was concentrated in the region 750 to 2300 cm$^{-1}$. However, a small amount of power was present to >3000 cm$^{-1}$ due to a fast leading edge pulse in the supercontinuum output. Strong peaks, such as the C-H stretch modes can therefore be seen. The raw SIP-CARS spectrum (green curve) has no NRB and the spectral lines are non-dispersive. Agreement of the peak positions between SIP-CARS and the spontaneous Raman spectrum (black curve) is evident. To correct the SIP-CARS peak heights for variation in the Stokes spectrum the sum spectrum, $\Sigma S$, of a glass coverslip was measured and used as an estimate of $I_S$ (red curve). The normalised SIP-CARS spectrum (blue curve) shows agreement with the spontaneous Raman measurements in terms of both spectral position and relative peak heights. In regions where $I_S$ was small the normalisation introduced noise, such as around the peak at 801 cm$^{-1}$ and the C-H stretch region near 3000 cm$^{-1}$. However, agreement between SIP-CARS and spontaneous Raman measurements is clear even in these regions. Noise blows up in regions where both $I_S$ and $\Delta S \simeq 0$; these have been masked for clarity.

The spontaneous Raman measurements were aquired on a Renishaw RM-100 microspectrometer in an epi-detection geometry (514 nm pump); $R_{\|}$ is the spectrum with incident and scattered polarisations mutually parallel, while $R_{\perp}$ is the spectrum with incident and scattered polarisations mutually perpendicular. The curve for comparison with SIP-CARS was formed as $R_{\|} - 3R_{\perp}$, as described in the main text.

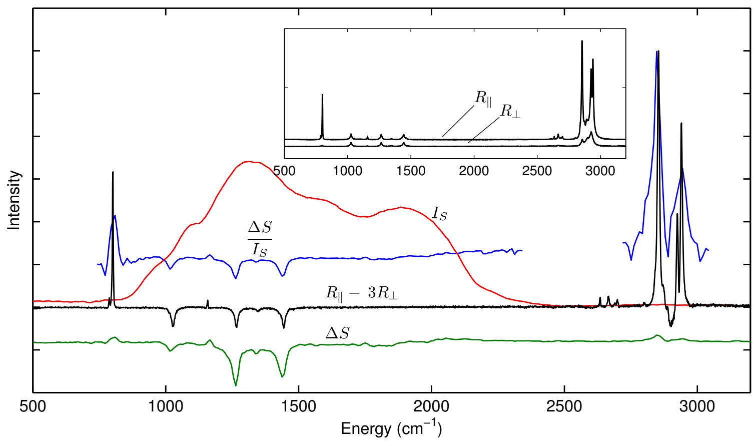


Figure 1: Full single-shot SIP-CARS spectrum of cyclohexane. Green: Raw SIP-CARS spectrum, $\Delta S$. Red: Sum spectrum, $\Sigma S$, of glass coverslip, used as an estimate of the spectral variation of Stokes beam, $I_S$. Blue: normalised SIP-CARS. Black: linear combination of polarised spontaneous Raman spectra, $R_{\|} - 3R_{\perp}$. Inset: parallel ($R_{\|}$) and perpendicular ($R_{\perp}$) polarised spontaneous Raman spectra.
